# Supplementary material for: Jigsaw: Large Language Models meet Program Synthesis
Source: arXiv:2112.02969 source file (2021-12-06)
Supplement: Supplementary file 1 [file appendix.tex]

In this section we describe the transformations that got learnt. 
\out{
\begin{figure}
    \centering
    \includegraphics[width=0.9\linewidth]{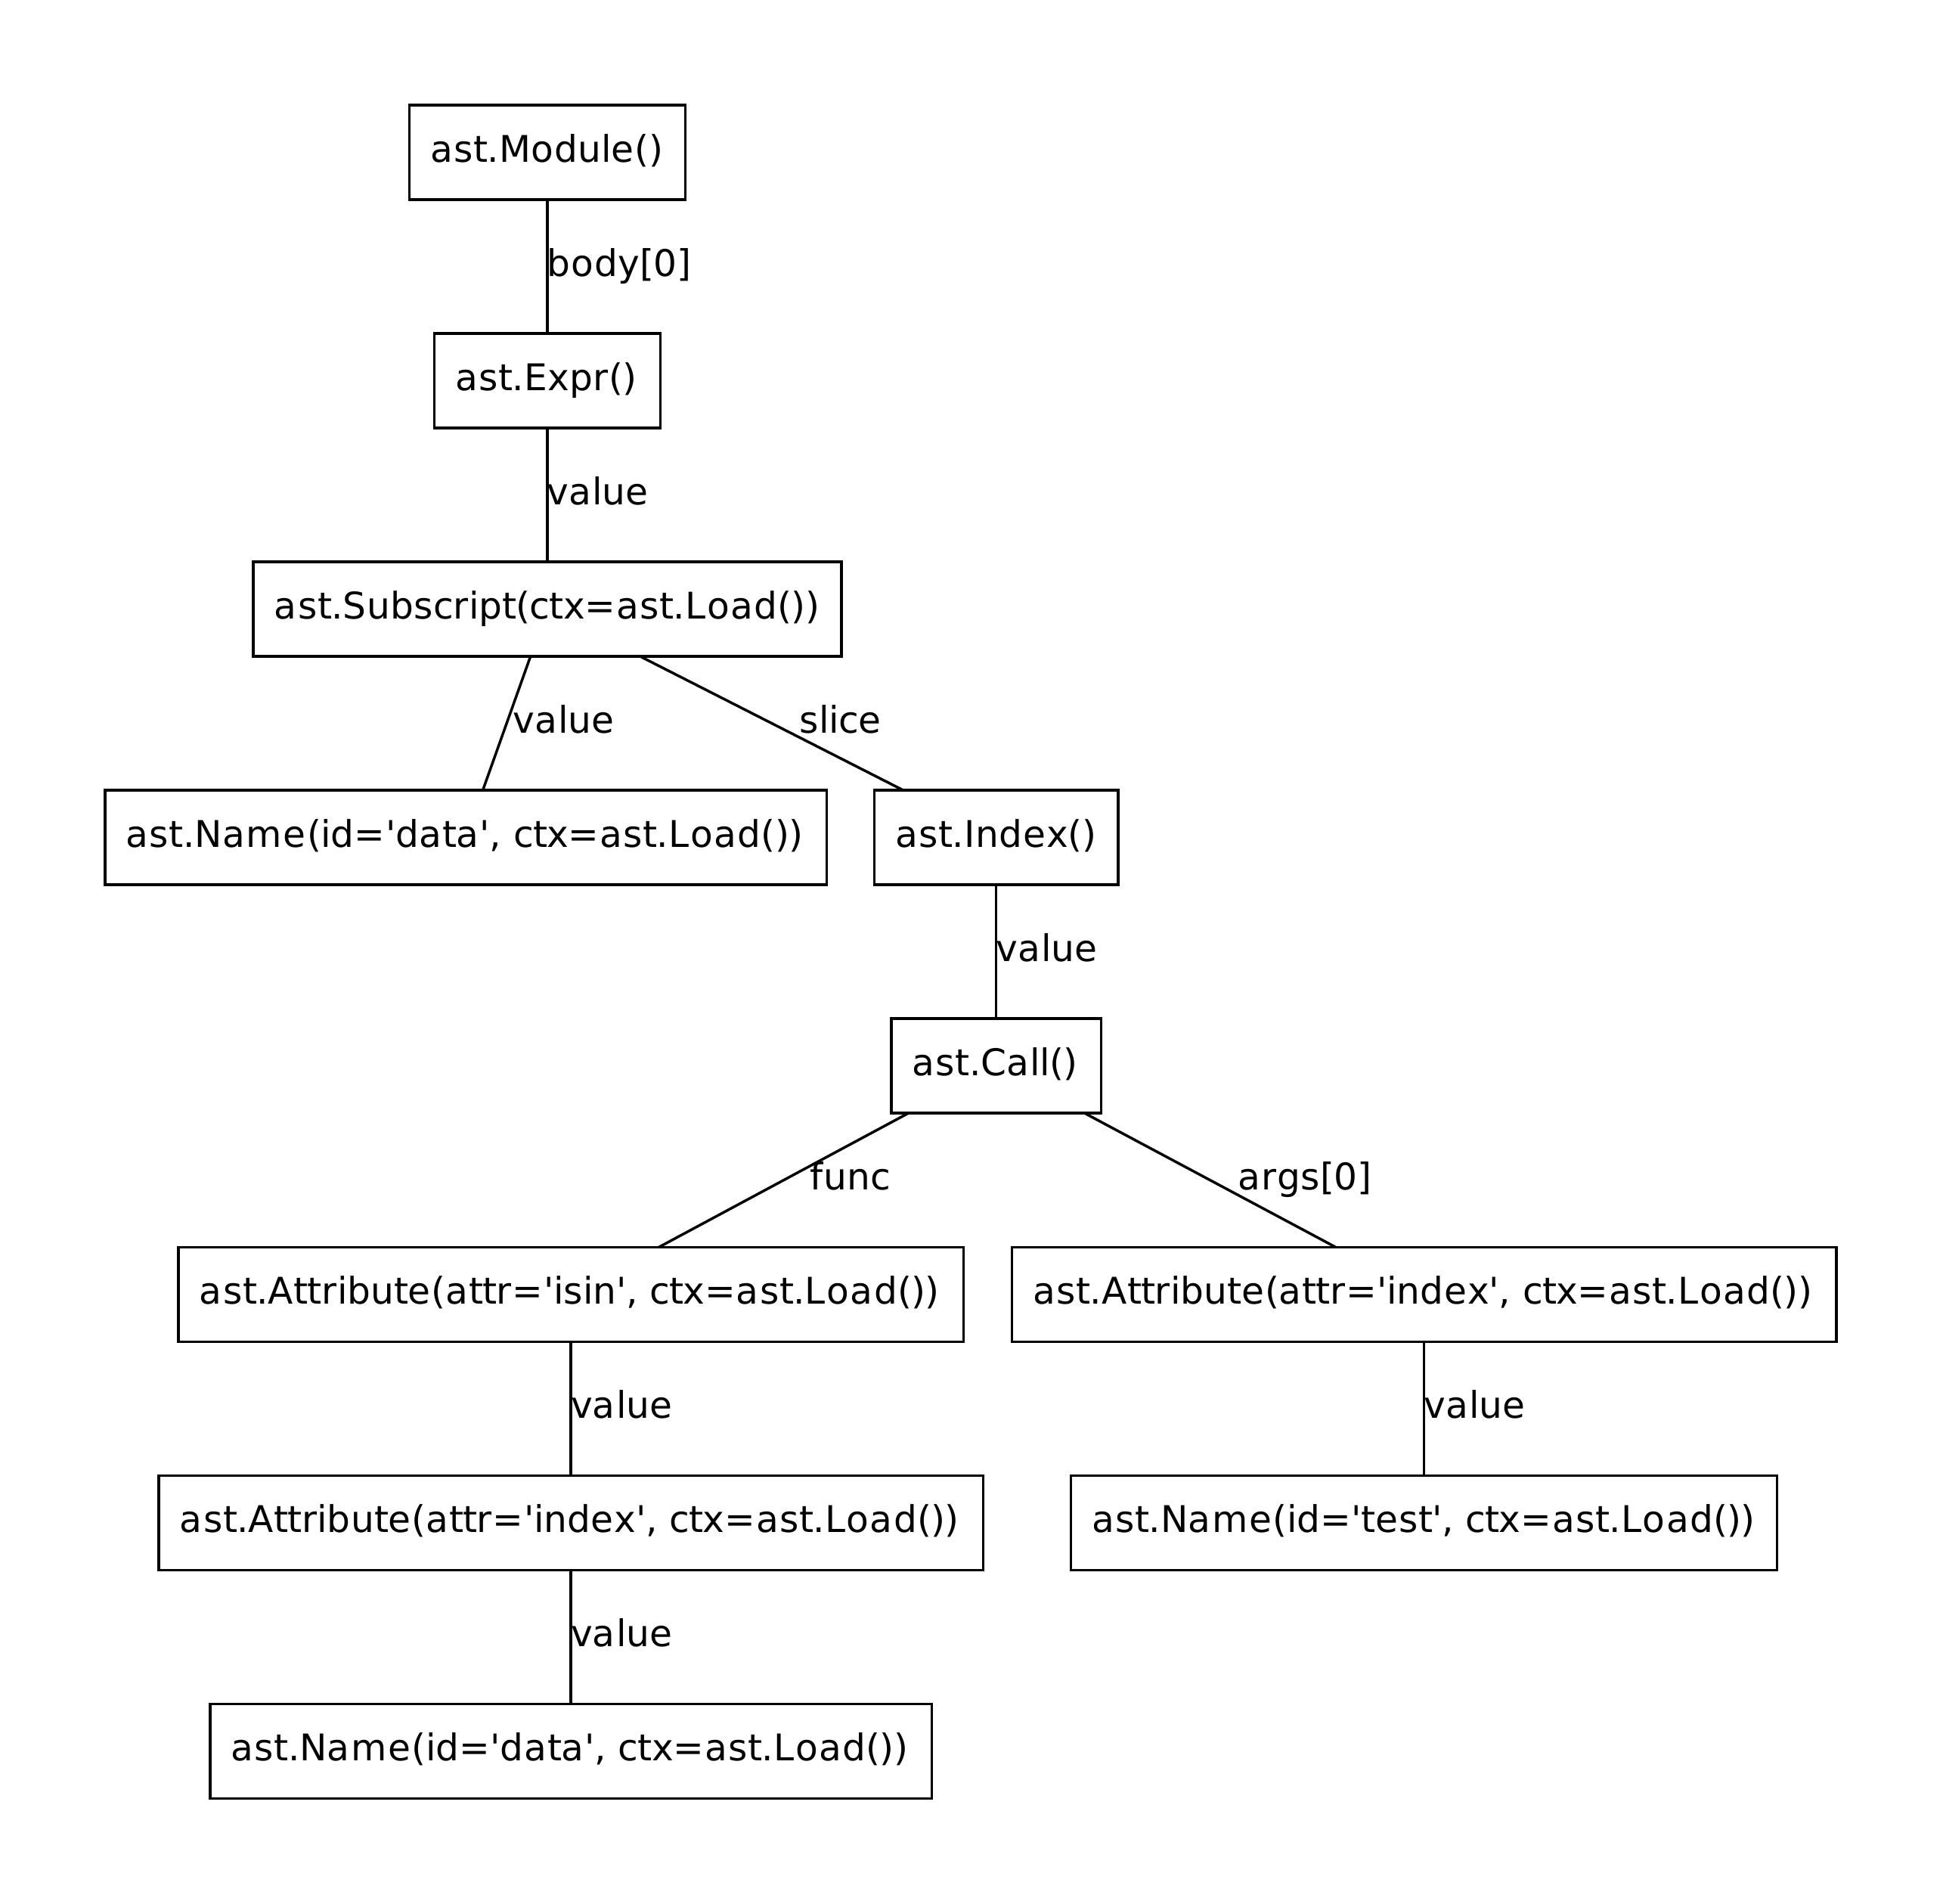}
    \caption{Caption}
    \label{fig:my_label}
\end{figure}

\begin{figure}
    \centering
    \includegraphics[width=0.9\linewidth]{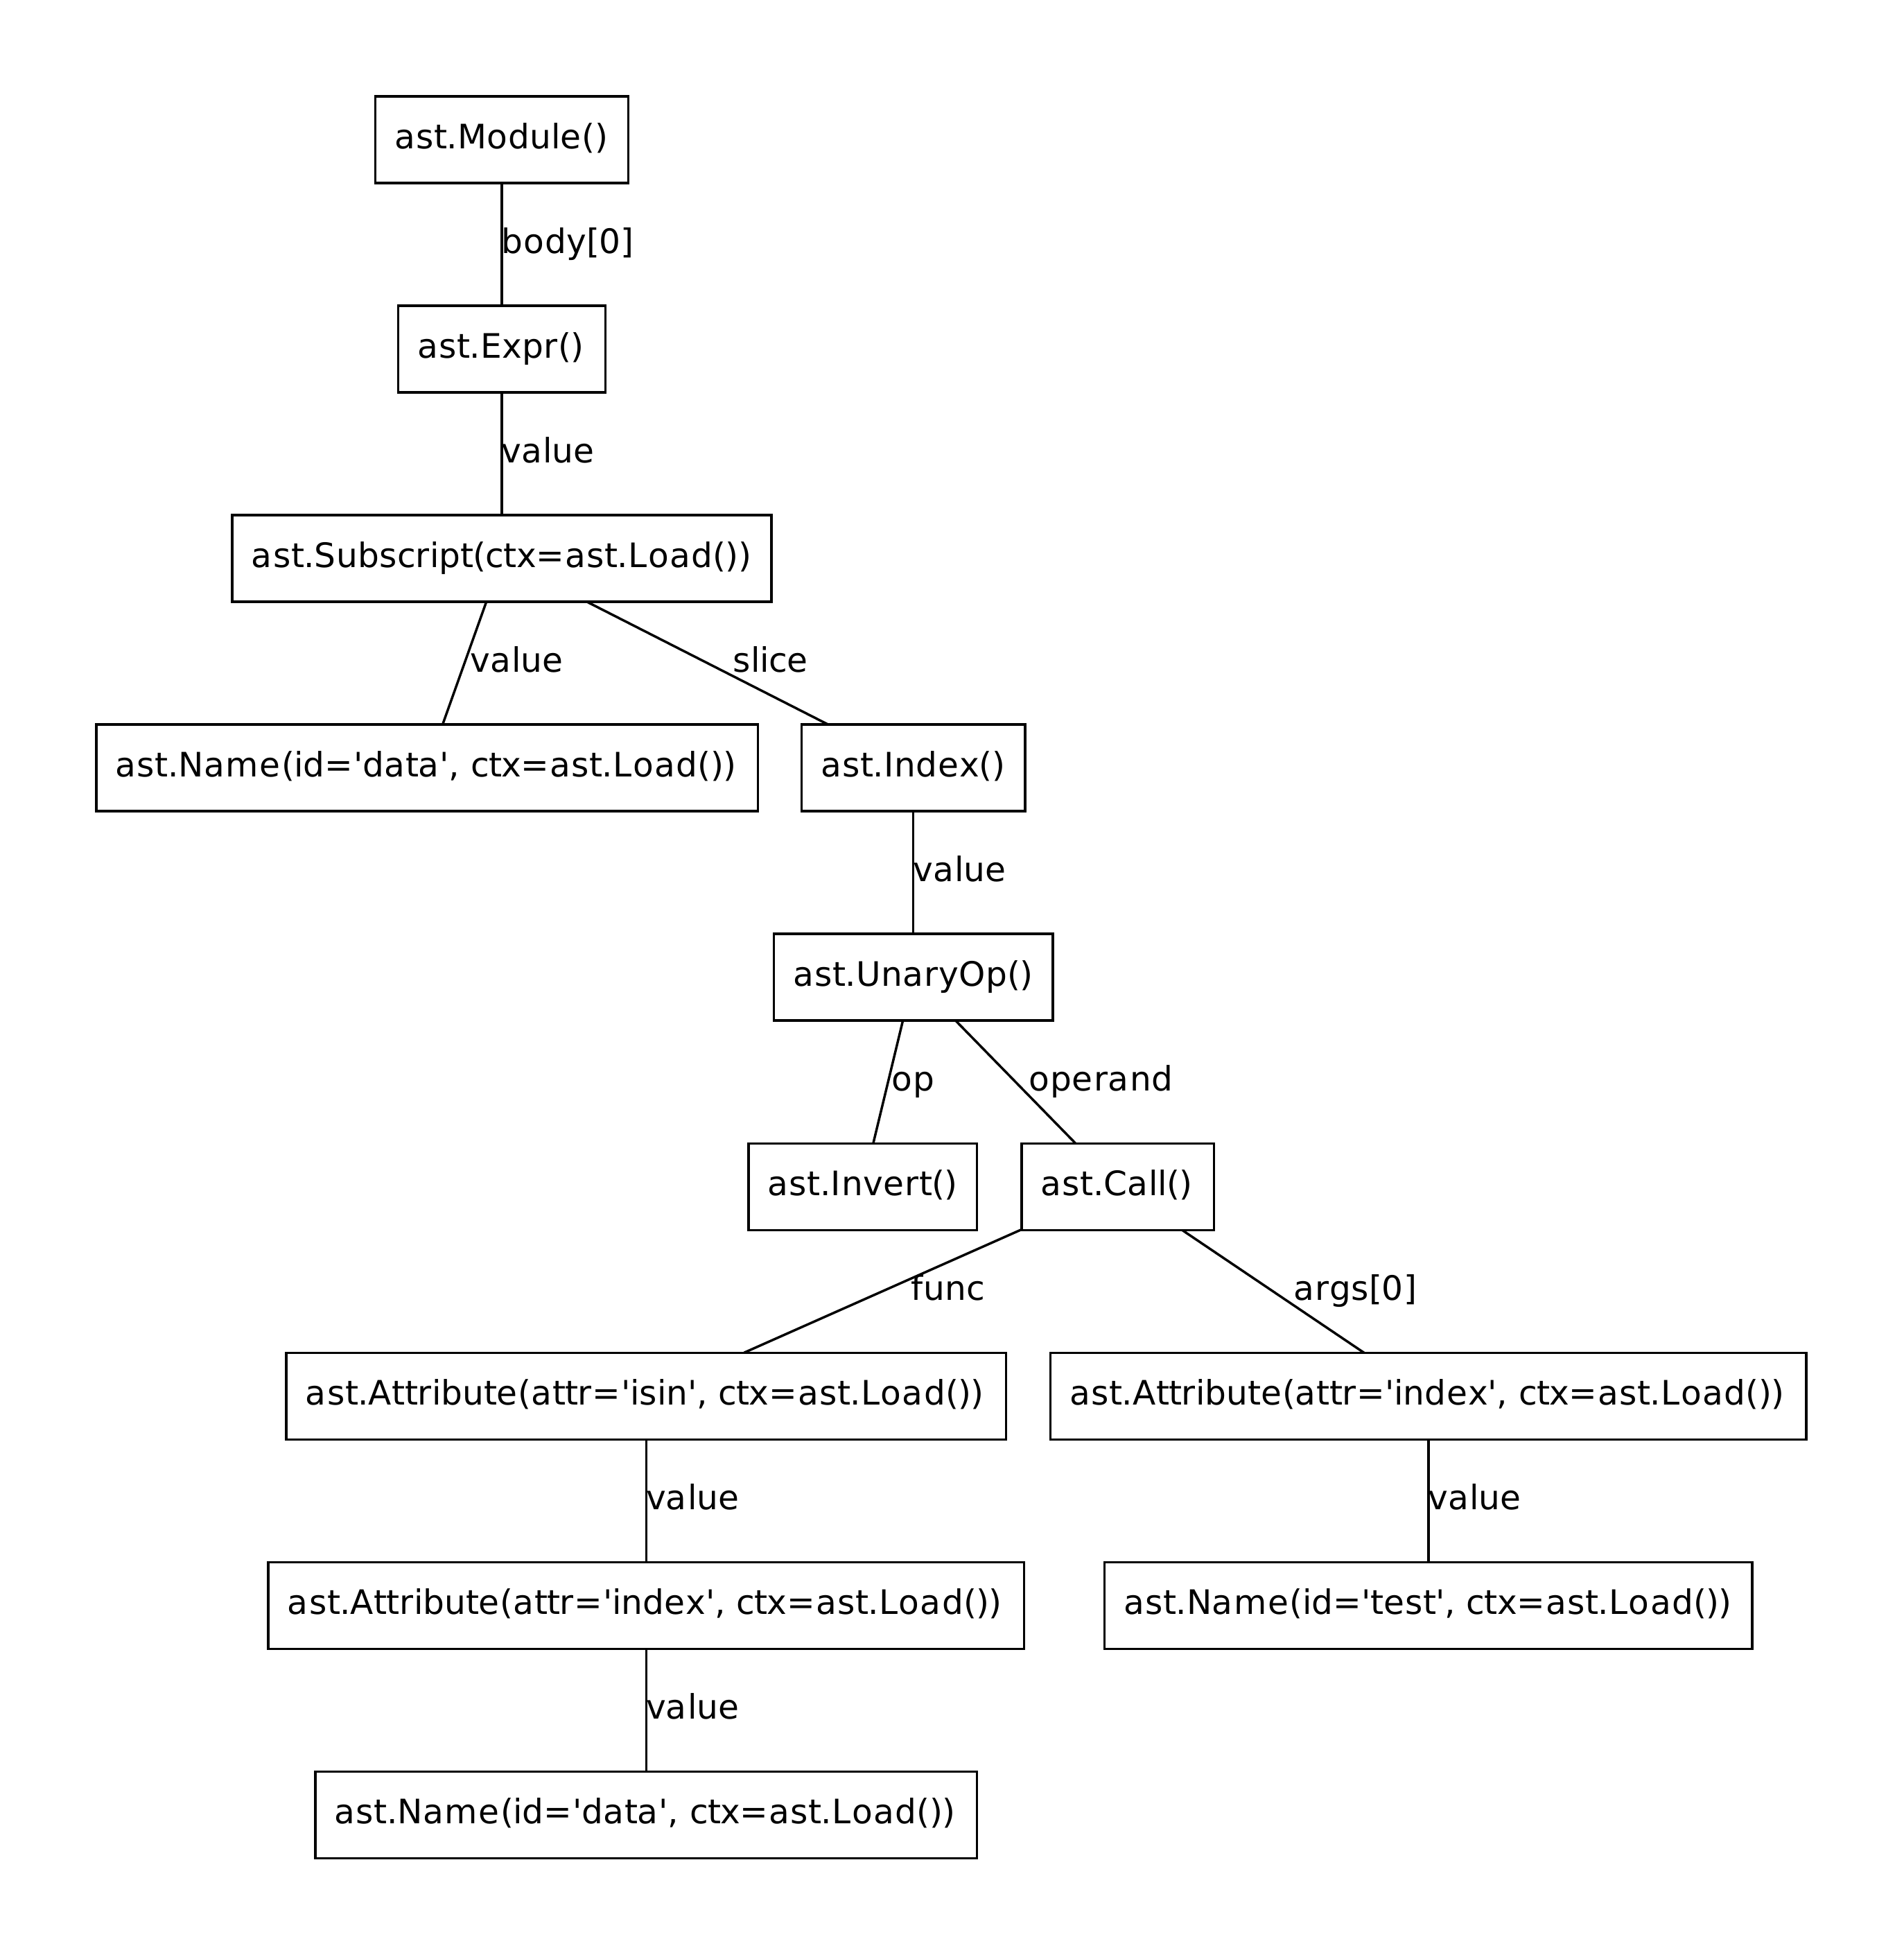}
    \caption{Caption}
    \label{fig:my_label}
\end{figure}
}
\begin{figure}
    \centering
    \includegraphics[width=0.9\linewidth]{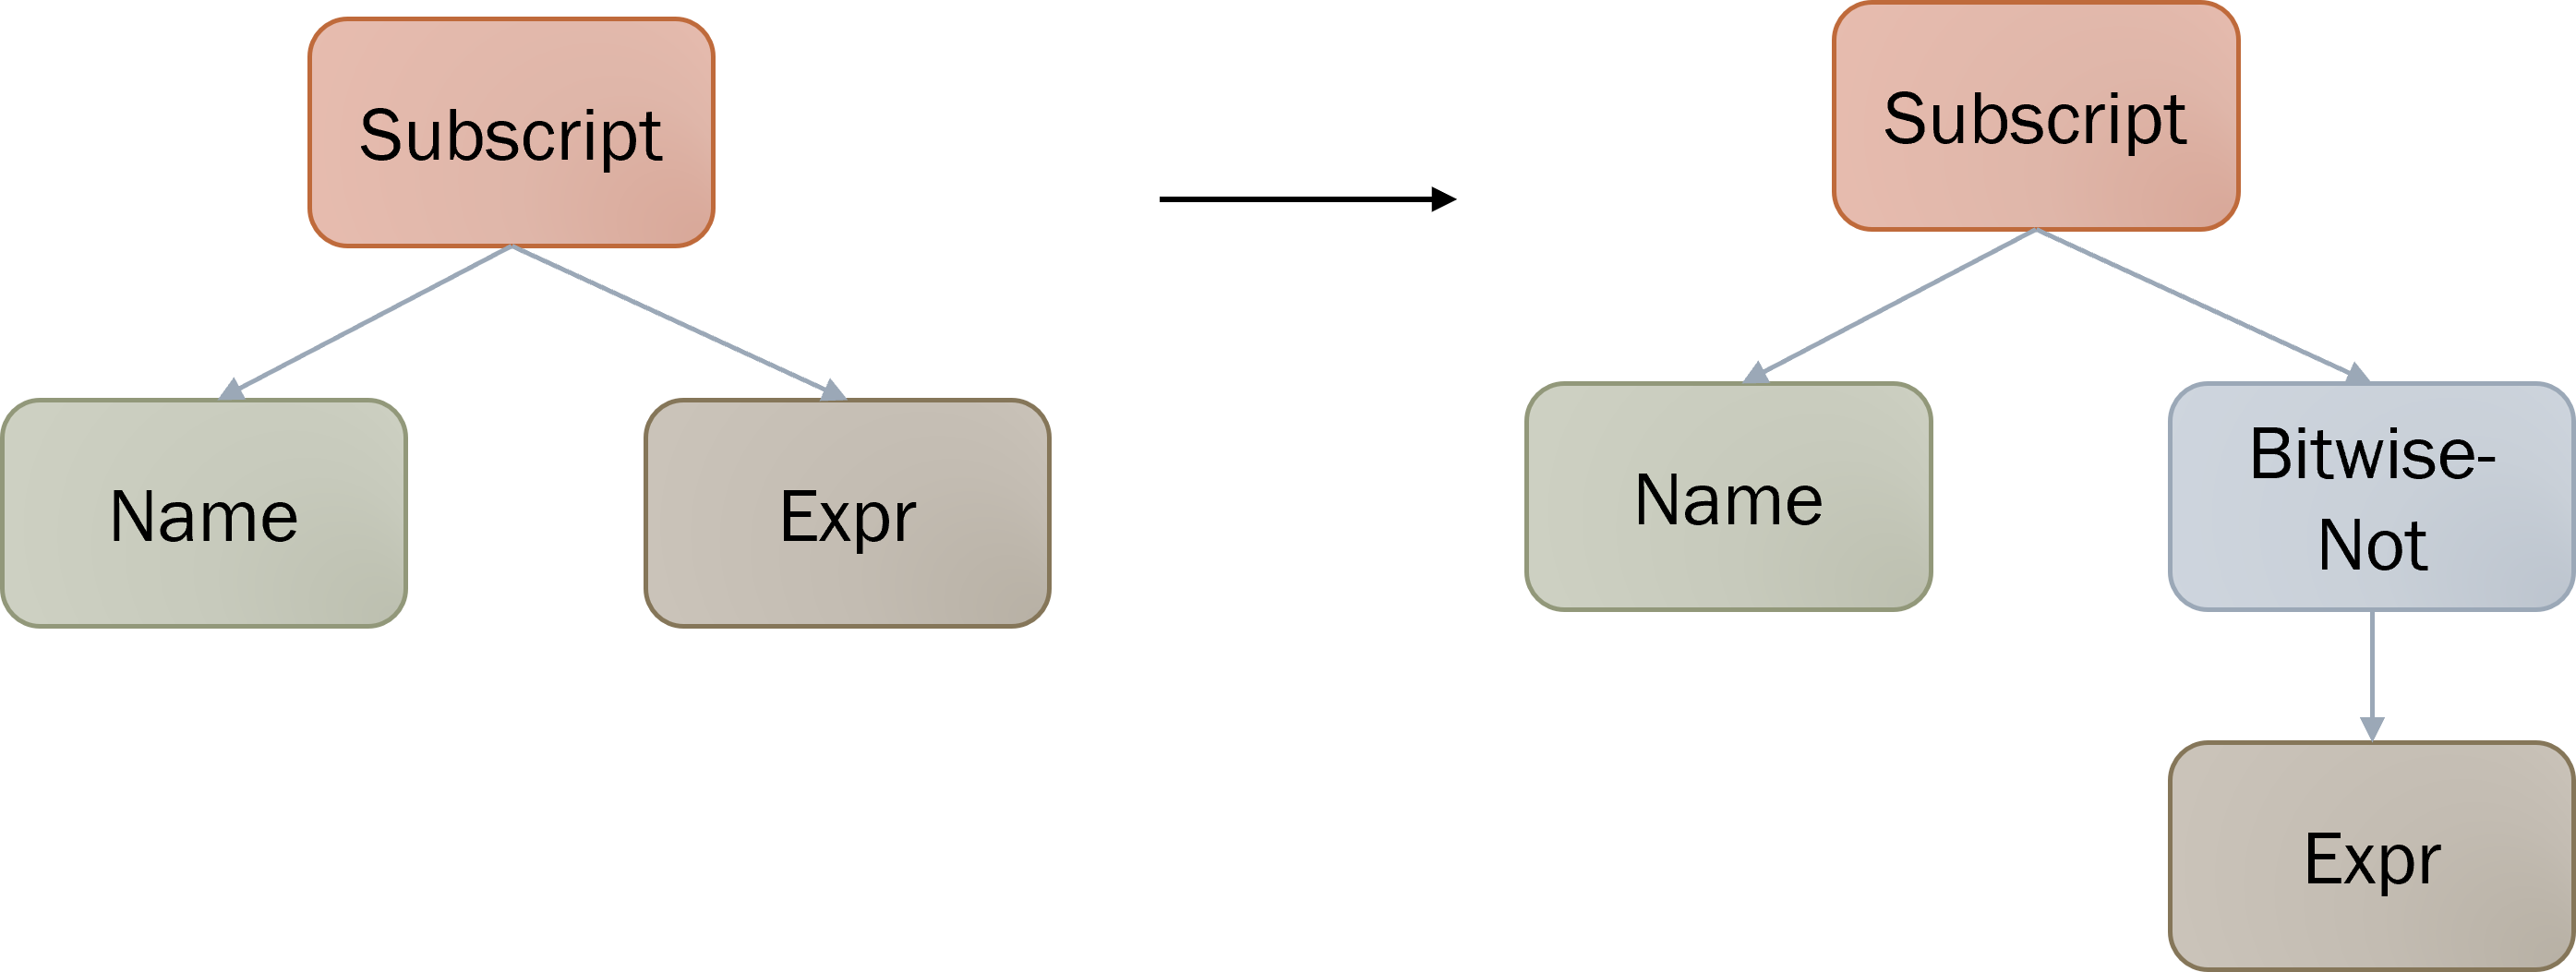}
    \caption{Caption}
    \label{fig:my_label}
\end{figure}

\begin{figure}
    \centering
    \includegraphics[width=0.9\linewidth]{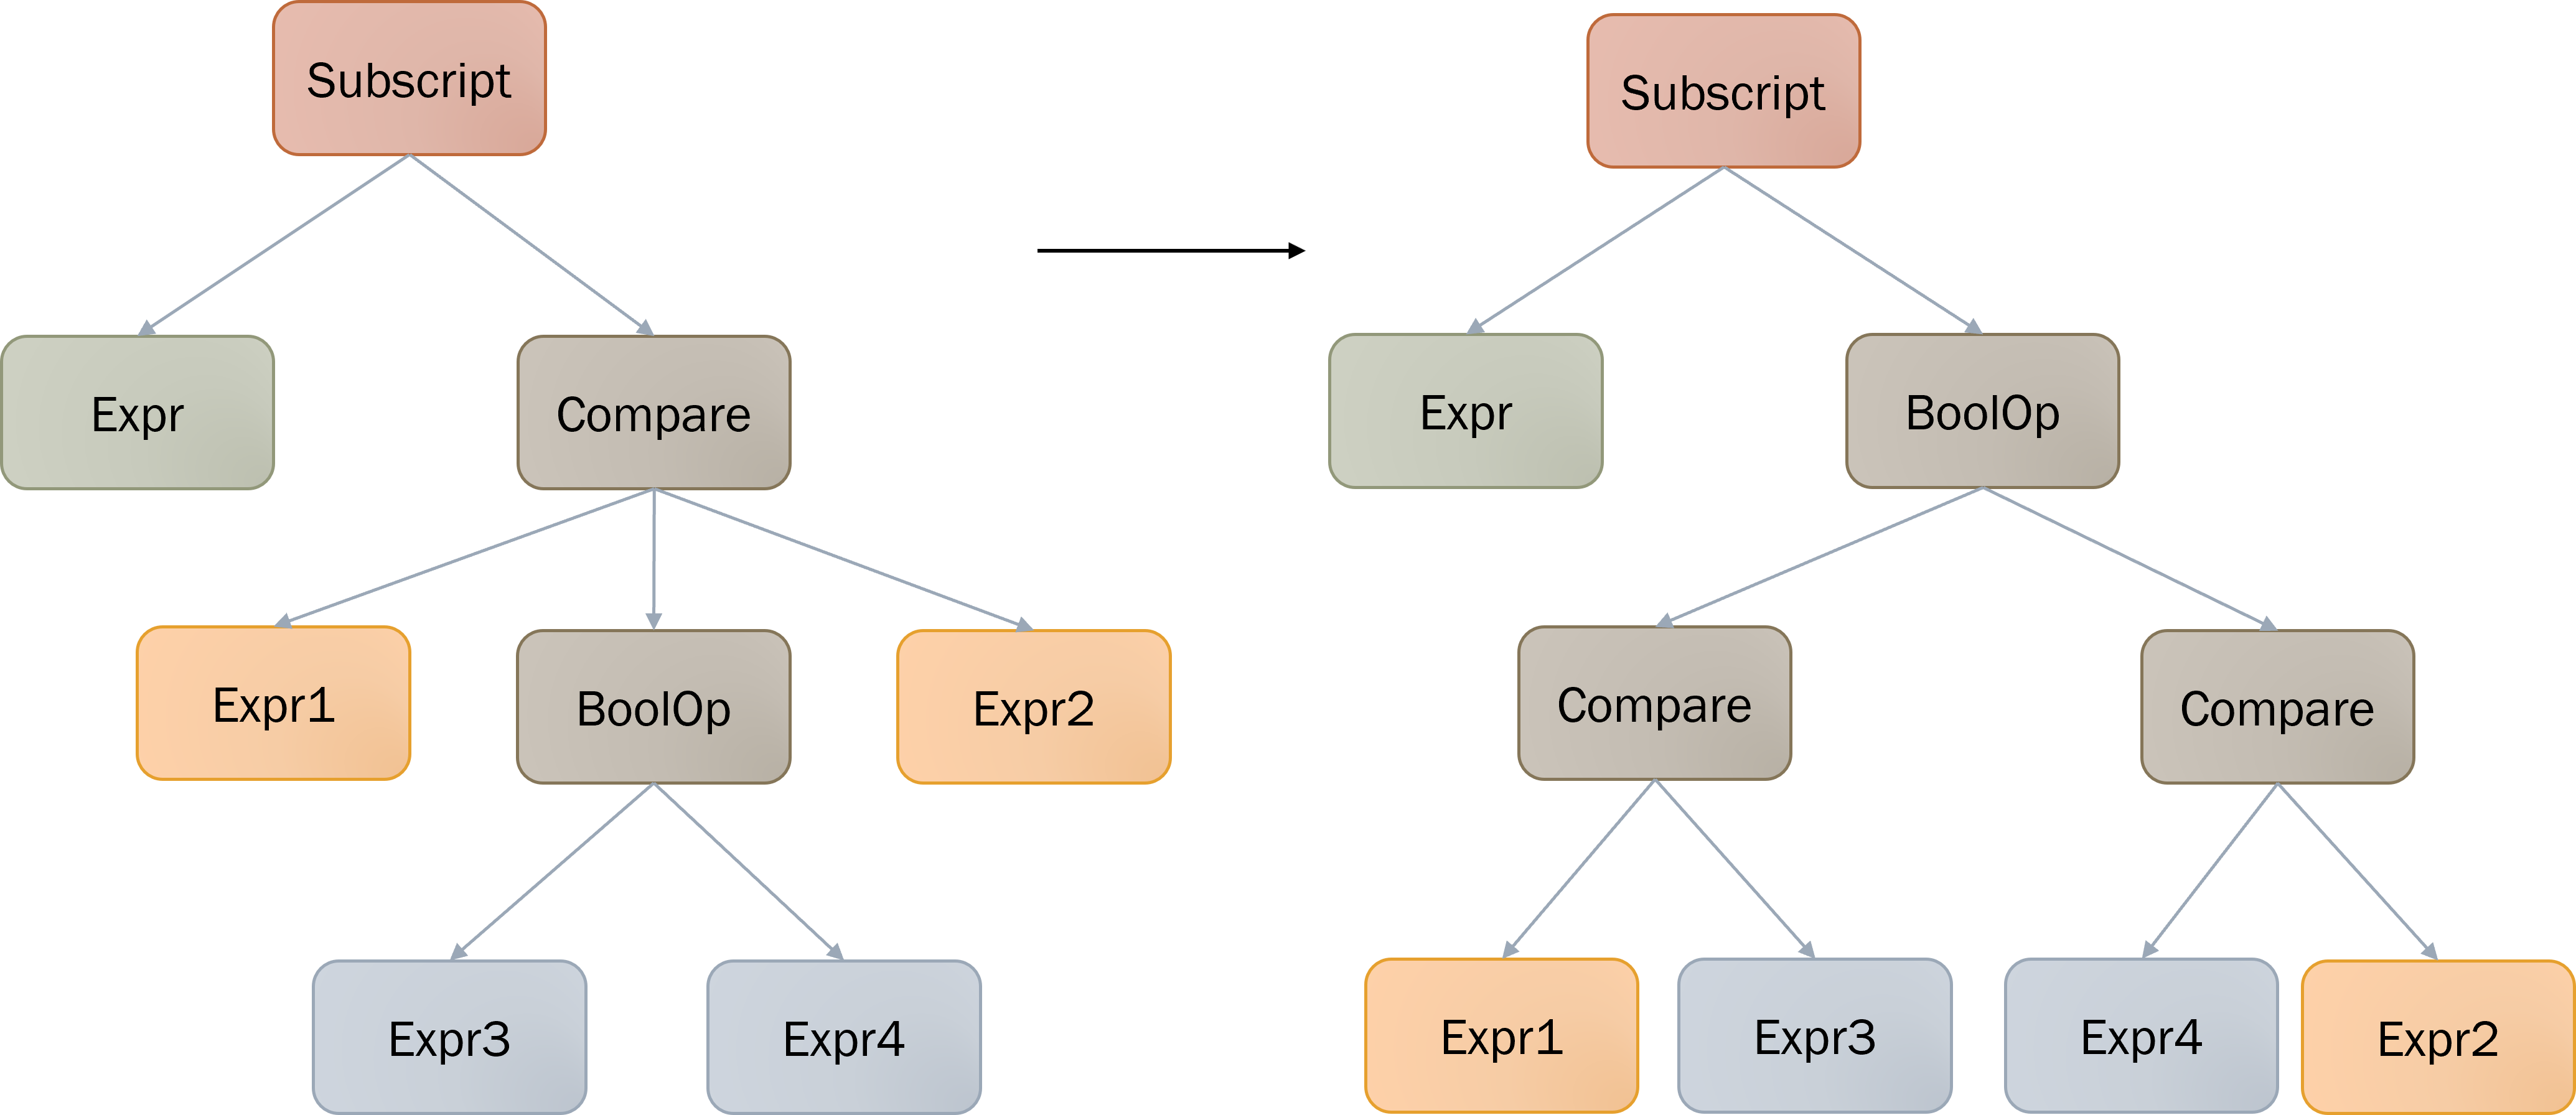}
    \caption{Caption}
    \label{fig:my_label}
\end{figure}

\begin{figure*}
    \centering
    \includegraphics[width=0.9\linewidth]{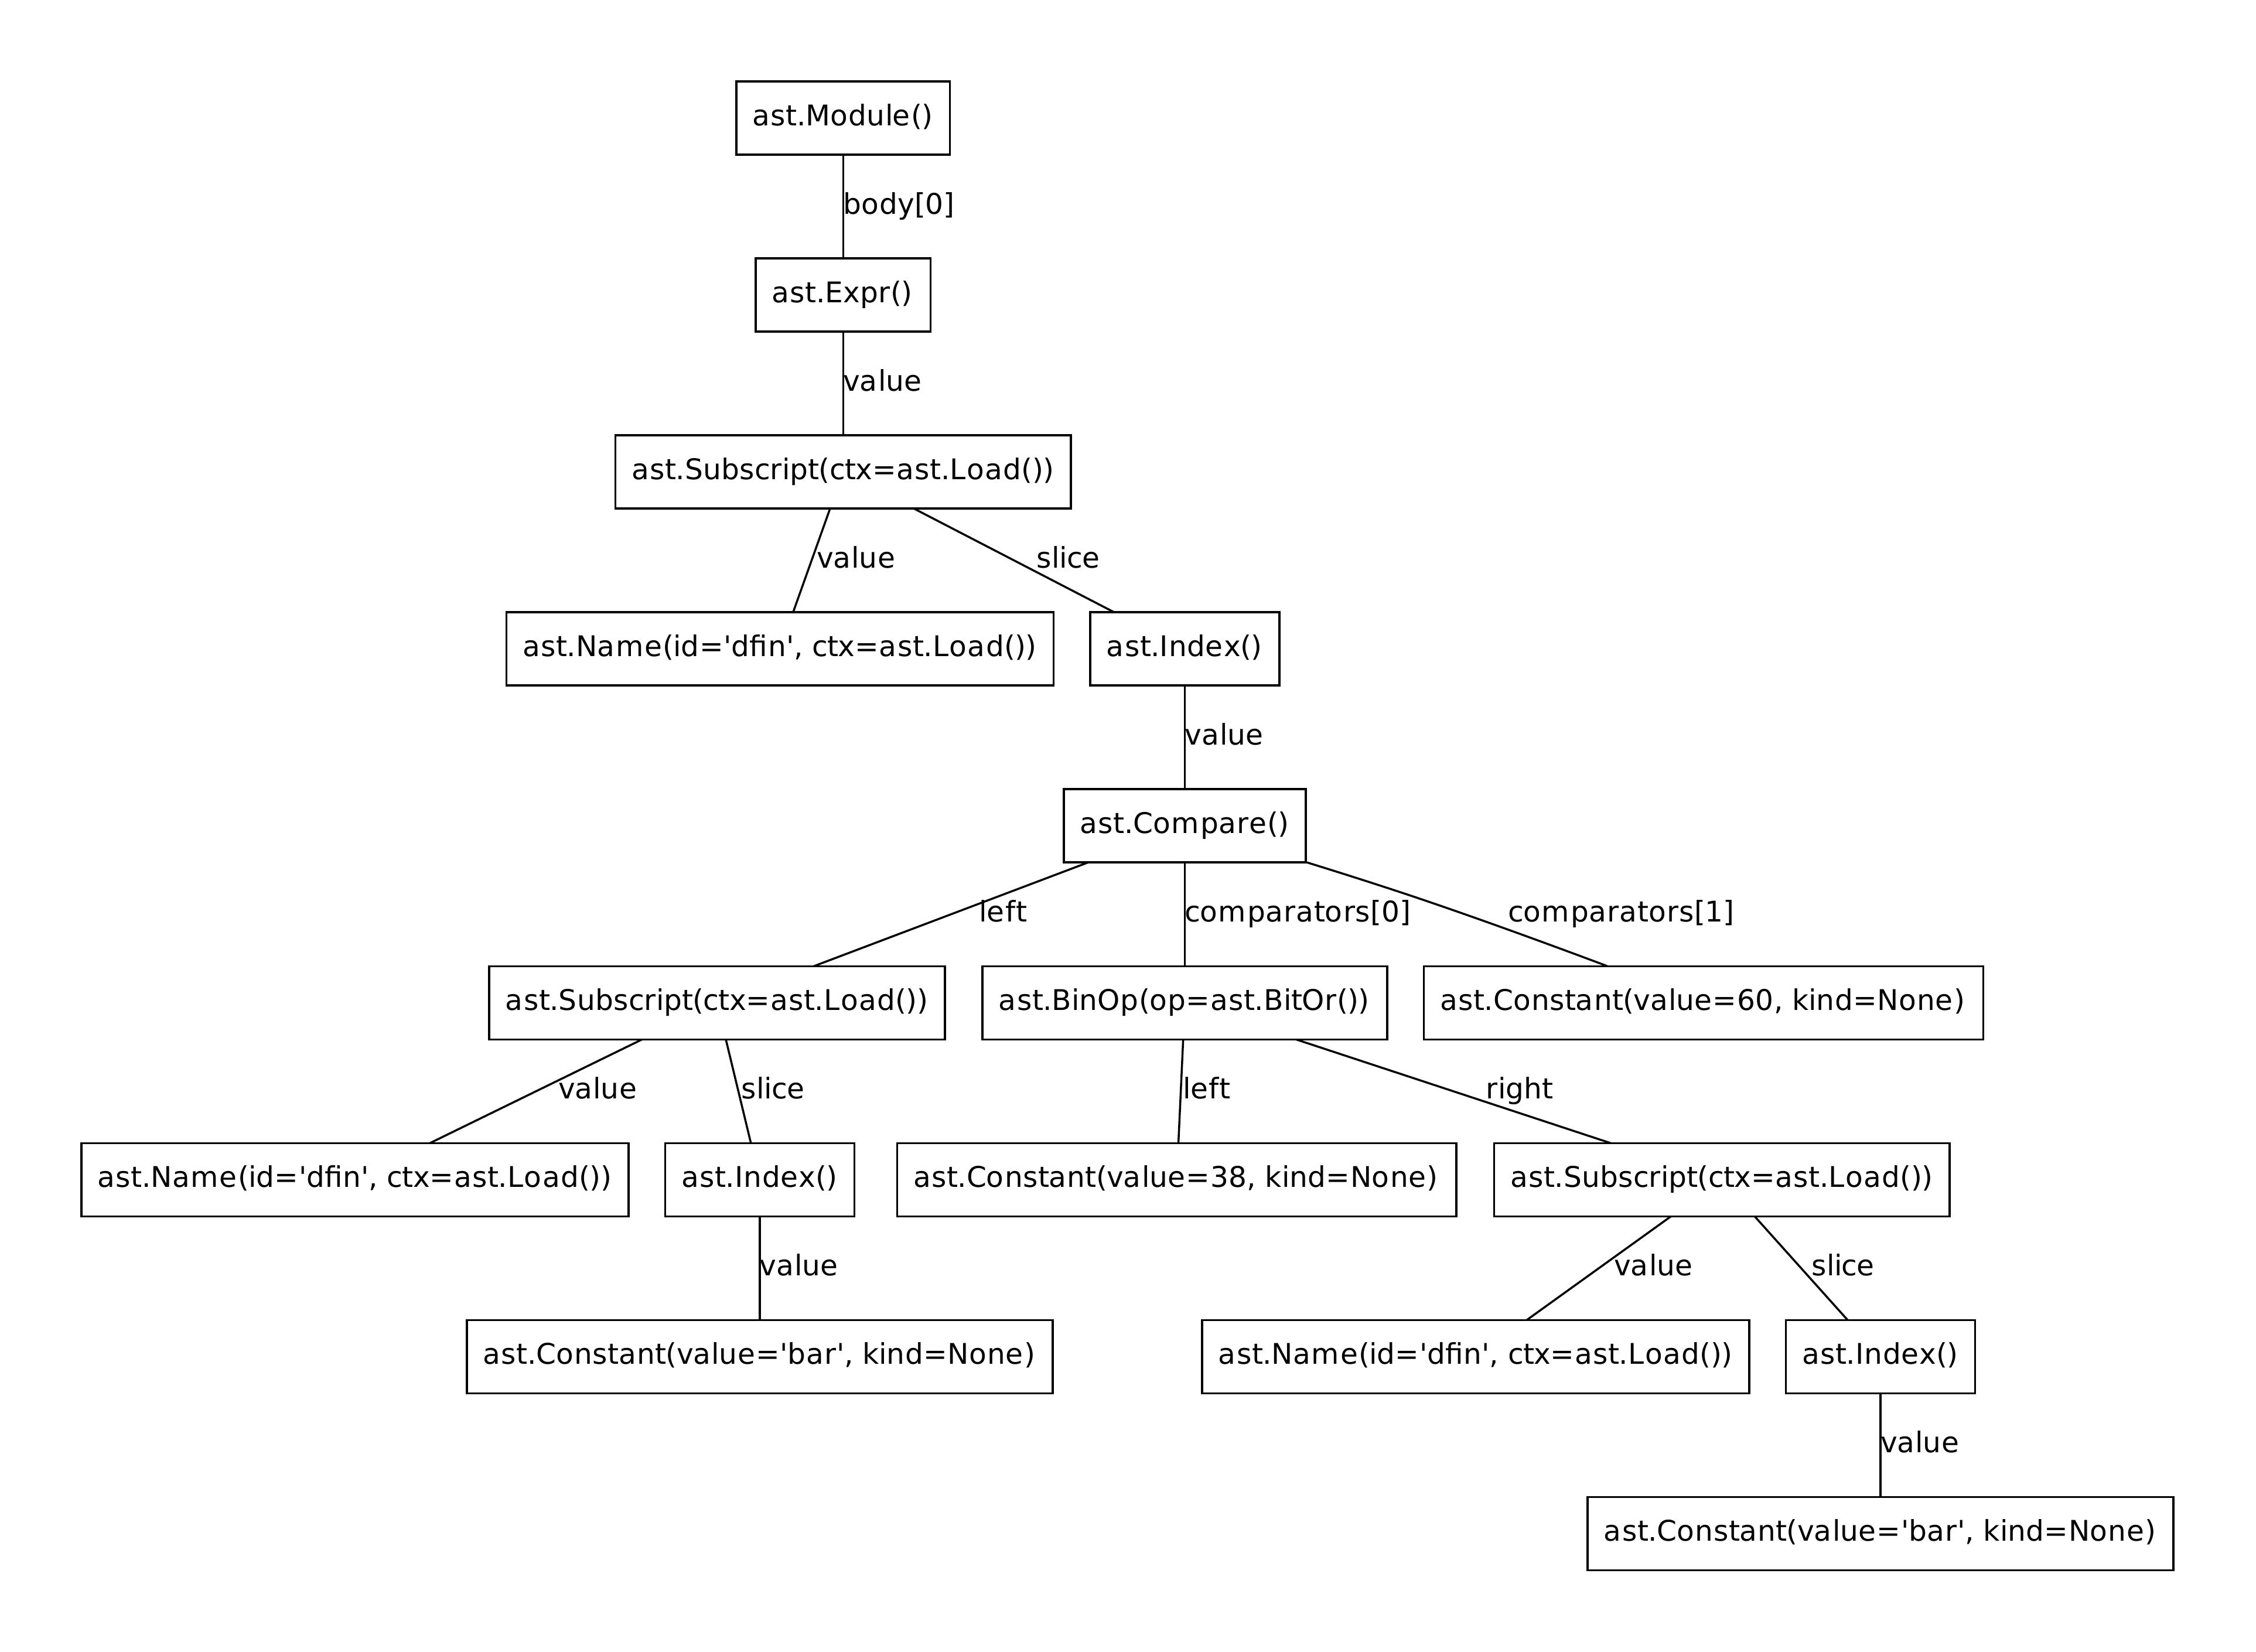}
    \caption{Caption}
    \label{fig:my_label}
\end{figure*}

\begin{figure*}
    \centering
    \includegraphics[width=0.9\linewidth]{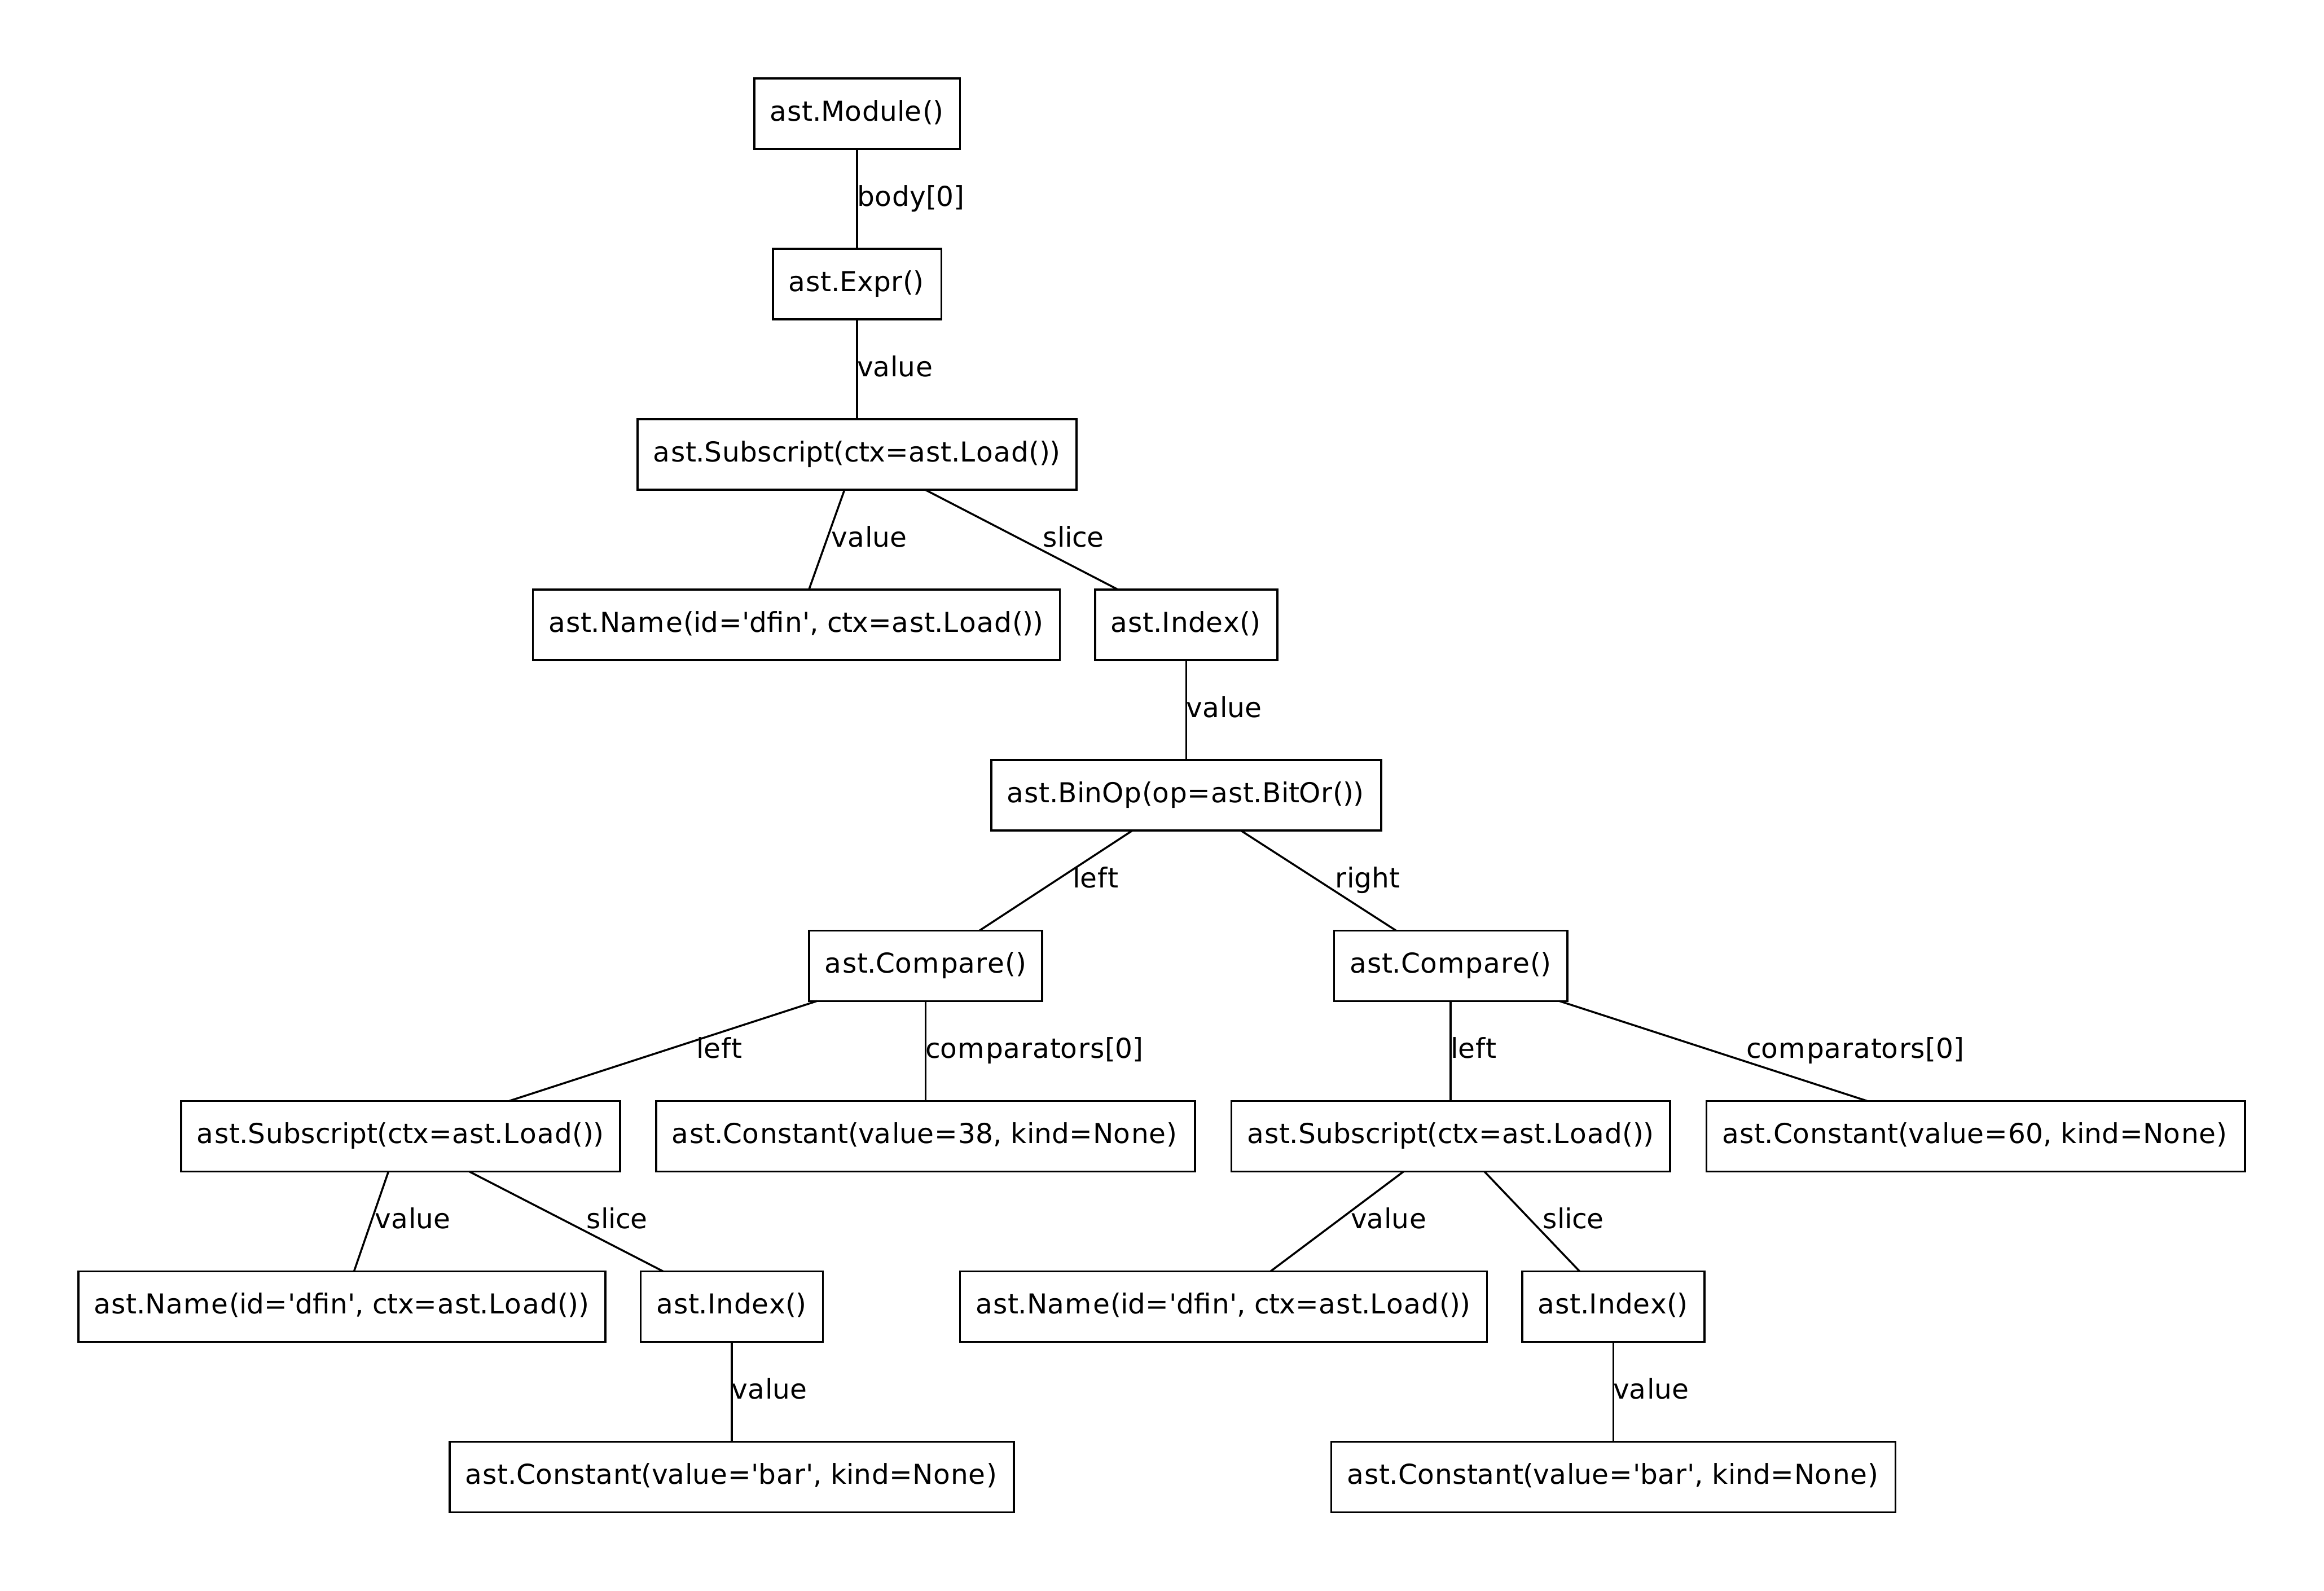}
    \caption{Caption}
    \label{fig:my_label}
\end{figure*}

\out{
\textbf{}\naman{\subsection{User experience} maybe in discussion?}
\spsays{Moving it behind for now}
\begin{table*}[t]
  \centering
  \begin{tabular}{p{8cm}p{8cm}}
    \toprule\\
    Positive & Negative\\
    \midrule\\
    "The overall experience was great! I had a lot of fun doing the questions and was able to solve most of the questions." & "The number of similar code output suggestions was a little overwhelming at first to go through each, and figure out the difference b/w the suggestions"\\
    "It can be used very easily for doing many tasks using pandas, and that makes it really easy for a non coder and saves time for others in looking up SO" & "The queries sometimes do not give correct code unless certain code-related keywords are used. Language used to communicate the task becomes very important"\\
    "It's fascinating, how Jigsaw entails the potential to remove the requirement to know "syntax and programming" for actual problem-solving and performing" & "I definitely struggled with forming well structured queries and validating the code-results that came to check if any of them could be correct" \\
    \bottomrule
  \end{tabular}
  \caption{User feedback}
  \label{Table:k}
\end{table*}
}
